# Supplementary material for: Design Space of Behaviour Planning for Autonomous Driving
Source: arXiv:1908.07931 source file (2019-08-21)
Supplement: Supplementary file 1 [file Appendix.tex]

\section*{Appendix: Local Planner Background}
%\label{sec:appendix}
%\subsection{Local Planner Background}
The local planner is the module of an autonomous driving software stack that is often the most dependent on the output of the behavioural planner. Because of this, when selecting the level of integration between the local planner and the behavioural planner, \added{presented in Section~\ref{sec:architecture},} a designer must exercise care when selecting a local planning algorithm. This is because different local planning algorithms can exploit different levels of behavioural planning interaction more effectively.
In the field of local planning for autonomous driving, there are currently three main types of motion planning algorithms\deleted{,} \added{---} variational \deleted{methods}, sampling-based \deleted{methods}, and lattice methods \cite{paden_cap_yong_yershov_frazzoli_2016}. \added{In what follows, we briefly describe each class to give an intuition regarding ``which local planning algorithm to choose given the behavior planner and accordingly the given interaction architecture''.}  \\

\subsubsection{Variational Methods}
Variational methods include the algorithms that optimize a trajectory function, which maps time steps to robot states, according to a cost functional. These cost functionals often include terms for both trajectory smoothness according to the kinodynamics of the robot, as well as for obstacle avoidance\cite{ratliff_zucker_bagnell_srinivasa_2009}. Because of the non-convex nature of these objective functions, convergence to feasible solutions can be an issue. To remedy this, convex approximations can be used to the functional, but this leaves the potential for sub-optimal solutions\cite{schulman_ho_lee_awwal_bradlow_abbeel_2013}. Despite this, these variational methods can be used in autonomous driving to generate driveable trajectories\cite{david_valencia_philippsen_bosshard_iagnemma_2017}, as well as to encode expressive behaviour in robot motion\cite{2018arXiv180900092Z}. One must always keep in mind the convergence issues present in these variational methods, however, which suits them to simpler objective functions.\\

\subsubsection{Sampling-Based Methods}
The goal of sampling-based methods is to sample candidate paths or trajectories from either the control space or workspace of the robot in order to reduce the search size during the motion planning process. Probabilistic algorithms are often efficient at finding collision-free paths in the workspace, but due to their asymptotic optimality\cite{karaman_frazzoli_2010}, running them for a short planning time can result in low-quality paths. In the context of autonomous driving, using workspace-conformal samples\cite{howard_green_kelly_ferguson_2008} can be useful for generating high-quality on-road trajectories. Recent work has discussed the possibility of learning different sampling distributions based on data\cite{ichter_harrison_pavone_2017}, which opens the avenue of having different sampling distributions to execute different driving behaviours.\\

\subsubsection{Lattice Methods}
In lattice planning methods, the planning search space is reduced by restricting motion to a fixed set of control actions, called a control set. If points in the workspace are thought of as graph vertices, and the control actions as edges, a control set implicitly defines a graph that can be searched for an optimal path\cite{pivtoraiko_knepper_kelly_2009}. By doing this, we can pre-compute the control set as well as search heuristics, which can greatly reduce the amount of online computation. An alternative to the lattice planner is the conformal lattice planner\cite{mcnaughton_urmson_dolan_lee_2011}, which connects laterally sampled points along the road to form a graph. These conformal planners have been shown to work well in on-road driving scenarios\cite{xu_wei_dolan_zhao_zha_2012}, and have been shown to leverage behavioural information effectively in the motion planning process, particularly in manoeuvre selection based on dynamic obstacle information\cite{gu_dolan_lee_2016}\cite{gu_2017}. In the non-conformal case, one could also use lattices for specific scenarios, such as parking lot manoeuvres~\cite{Urmson-2008-10020}.
